# Supplementary material for: Evidence of absorption dominating over scattering in light attenuation by nanodiamonds
Source: arXiv:1812.03512 ancillary file (2019-07-26)
Supplement: Supplementary file 1 [file Supplementary___nanodiamonds.pdf]

# Evidence of absorption dominating over scattering in light attenuation by nanodiamonds

S. V. Koniakhin,<sup>1,2,3,\*</sup> M. K. Rabchinskii,<sup>2</sup> N. A. Besedina,<sup>2,3</sup>  
L. V. Sharonova,<sup>2</sup> A. V. Shvidchenko,<sup>2</sup> and E. D. Eidelman<sup>2,4</sup>

<sup>1</sup>*Institut Pascal, PHOTON-N2, University Clermont Auvergne,  
CNRS, 4 avenue Blaise Pascal, 63178 Aubière Cedex, France*

<sup>2</sup>*Ioffe Institute, 194021 St. Petersburg, Russia*

<sup>3</sup>*St. Petersburg Academic University - Nanotechnology Research and Education  
Centre of the Russian Academy of Sciences, 194021 St. Petersburg, Russia*

<sup>4</sup>*St. Petersburg Chemical Pharmaceutical Academy, 197022 St. Petersburg, Russia*

Supplementary data, Jyly 2019

---

\* [kon@mail.ioffe.ru](mailto:kon@mail.ioffe.ru)

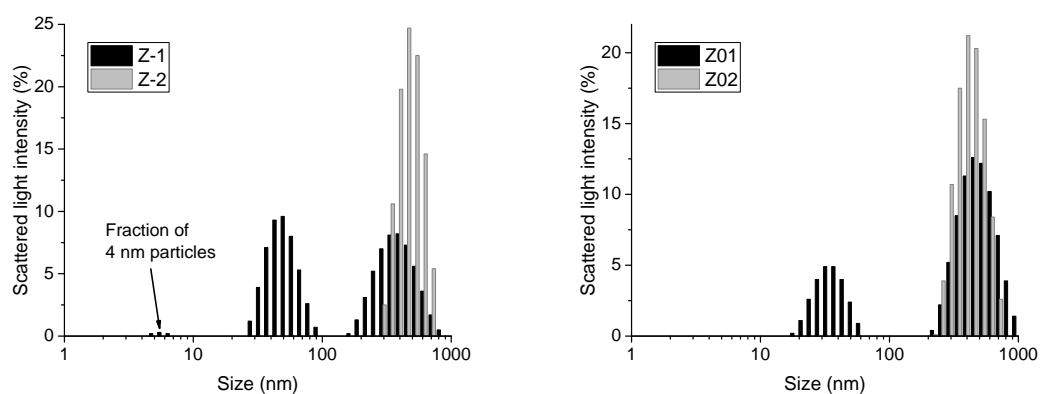

Figure S1. Distribution by scattered light intensity for Z- and Z0 samples obtained by DLS.

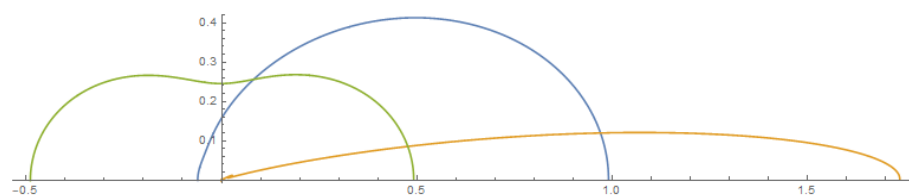

Figure S2. Scattering indicatrix for various sized nanodiamonds. Green color is for primary 4 nm crystallites, blue color is for 90 nm agglomerates and yellow is for 700 nm agglomerates. Wavelength in vacuum is 250 nm.

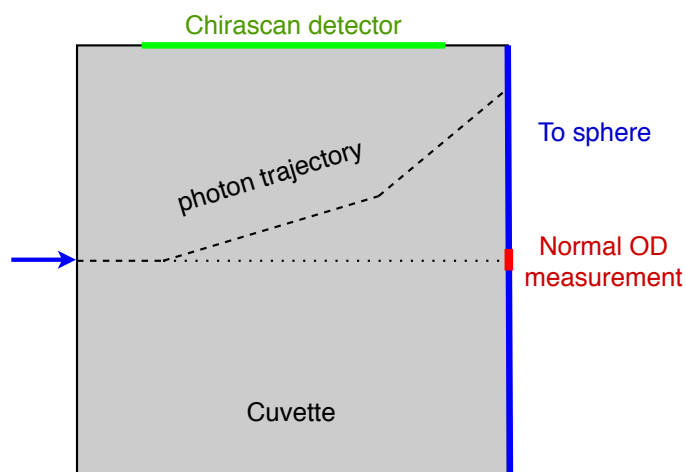

Figure S3. Simulation scheme. Top view of the simulation box.

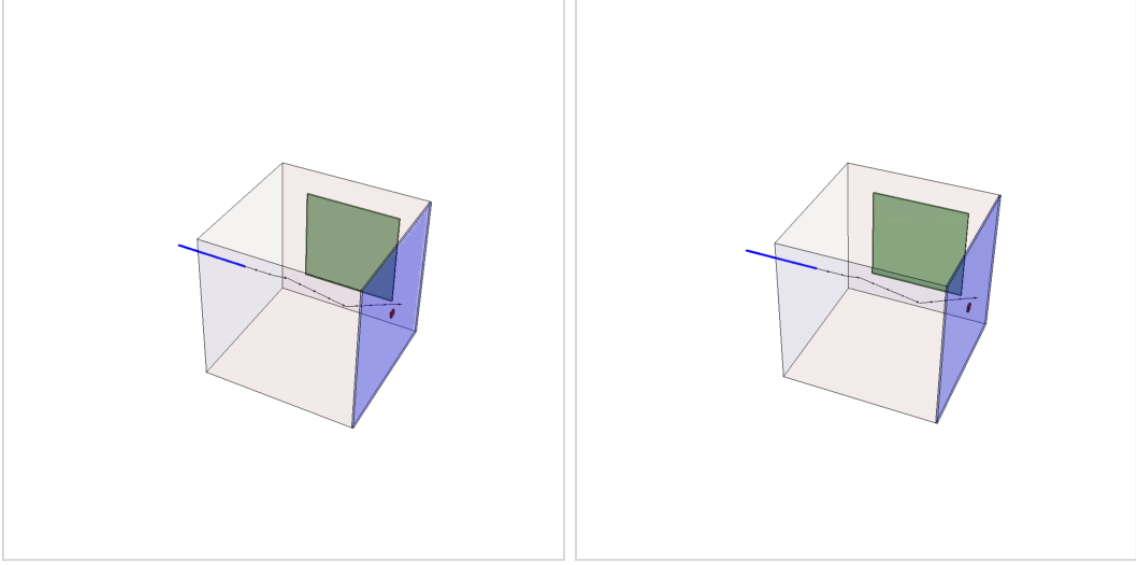

Figure S4. Crosseyed stereo 3D image of a typical photon trajectory in Z+2 hydrosol. Green rectangle is a "Chirscan detector". Blue wall corresponds to integrating sphere and small red rectangle is for Abs measurements without integrating sphere.

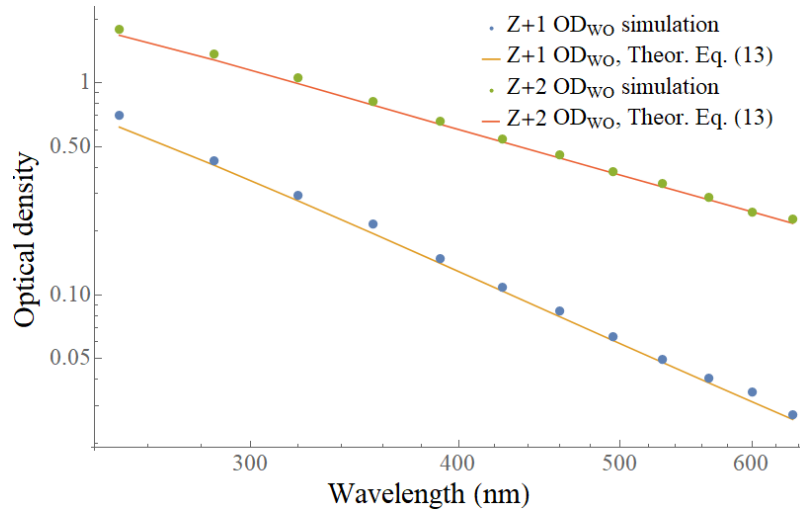

Figure S5. Comparison of Abs spectra obtained theoretically via Eq. (13) and on the basis of photon random walks simulation for DND Z+1 and Z+2. Vanishing difference is due to finite step size  $dl$ .

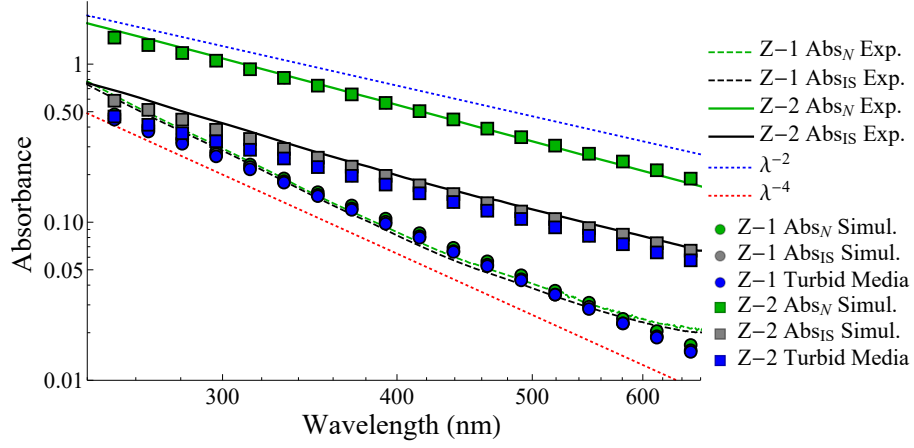

Figure S6. The obtained with photon random walk simulation Abs spectra with and without sphere (depicted with markers) and the experimentally measured Abs spectra of Z-1 (dashed curves) and Z-2 (solid curves) samples with (black curves) and without sphere (green curves). The predictions of the theory of light propagation in turbid media for Abs spectra with integrating sphere are shown with the blue markers. The red dashed curve shows the  $\lambda^{-4}$  function corresponding to Rayleigh scattering and the blue dashed is for  $\lambda^{-2}$ .

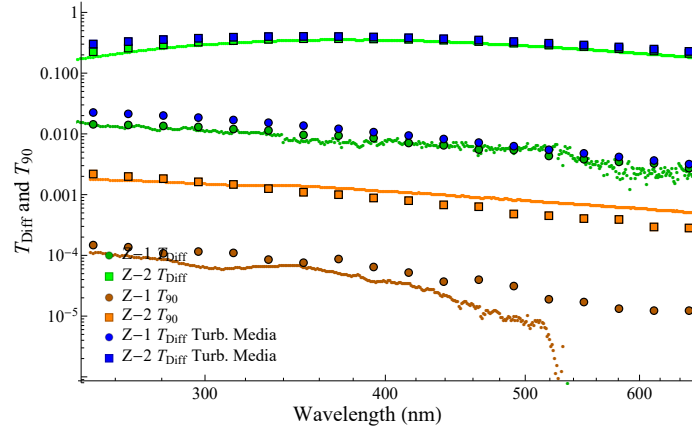

Figure S7. The results of photon random walk simulations for scattering efficiency in terms of  $T_{\text{FS}}(\lambda)$  (green colors) and  $T_{90}(\lambda)$  (orange colors) are shown with markers. Circles are for Z-1 and squares are for Z-2 sample. The experimental spectra are given by dense points. Experimental  $T_{\text{FS}}(\lambda)$  spectra were obtained on the basis of Abs measurements with and without sphere using Eq. (4) and experimental  $T_{90}(\lambda)$  spectra were obtained from 90 degree scattering experiment on Chiriscan device using Eq. (5). Blue markers denote the results of the theory of light propagation in turbid media.

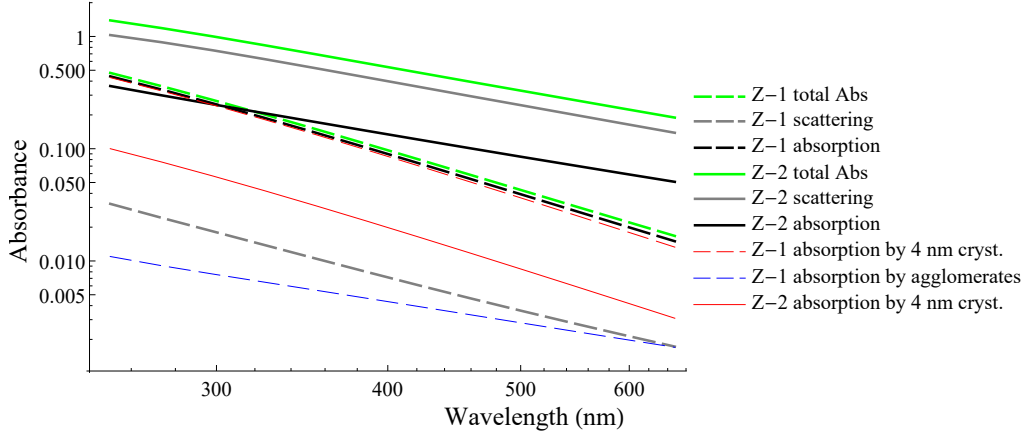

Figure S8. Decomposition of Abs spectra to scattering and absorption based on the Eqs. (11) and (12). Solid curves are for Z+2 and dashed curves are for Z-1 samples. Green color is for total Abs, gray color is for scattering and black color is for absorption. For supernatant Z+1 the contribution to absorption from primary crystallites (red color) and agglomerates (blue color) is given. For precipitate Z-2 both scattering and absorption is governed mainly by agglomerates.

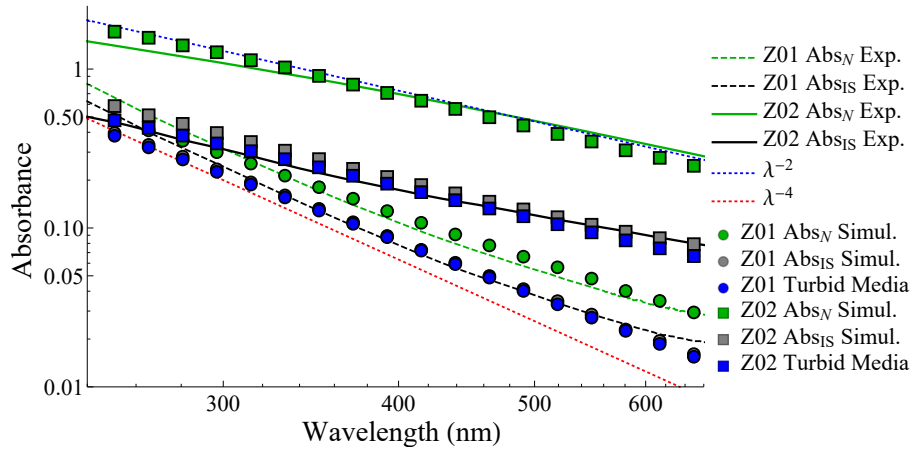

Figure S9. The obtained with photon random walk simulation Abs spectra with and without sphere (depicted with markers) and the experimentally measured Abs spectra of Z01 (dashed curves) and Z02 (solid curves) samples with (black curves) and without sphere (green curves). The predictions of the theory of light propagation in turbid media for Abs spectra with integrating sphere are shown with the blue markers. The red dashed curve shows the  $\lambda^{-4}$  function corresponding to Rayleigh scattering and the blue dashed is for  $\lambda^{-2}$ .

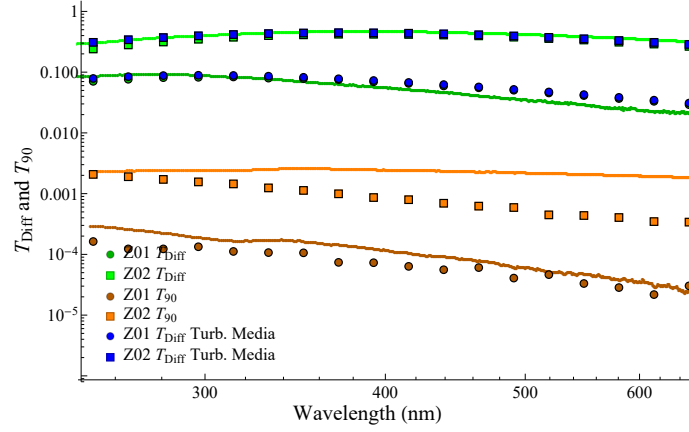

Figure S10. The results of photon random walk simulations for scattering efficiency in terms of  $T_{FS}(\lambda)$  (green colors) and  $T_{90}(\lambda)$  (orange colors) are shown with markers. Circles are for Z01 and squares are for Z02 sample. The experimental spectra are given by dense points. Experimental  $T_{FS}(\lambda)$  spectra were obtained on the basis of Abs measurements with and without sphere using Eq. (4) and experimental  $T_{90}(\lambda)$  spectra were obtained from 90 degree scattering experiment on Chirascan device using Eq. (5). Blue markers denote the results of the theory of light propagation in turbid media.

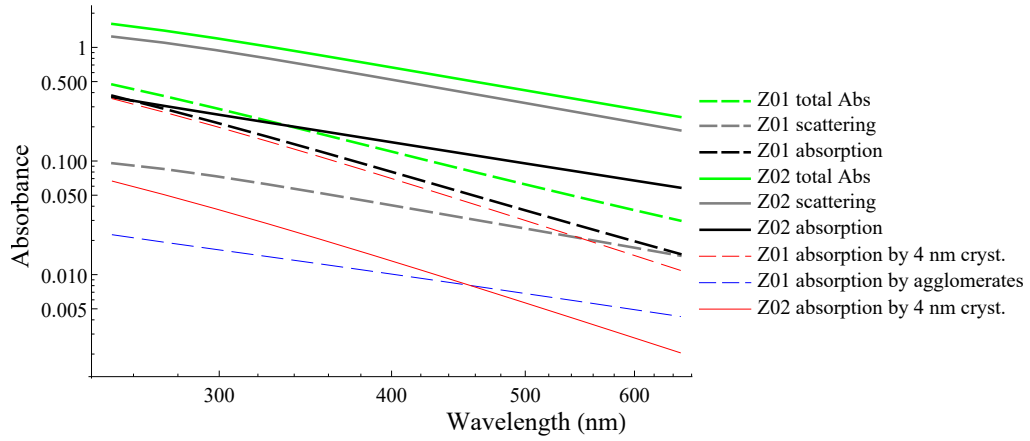

Figure S11. Decomposition of Abs spectra to scattering and absorption based on the Eqs. (11) and (12). Solid curves are for Z+2 and dashed curves are for Z01 samples. Green color is for total Abs, gray color is for scattering and black color is for absorption. For supernatant Z01 the contribution to absorption from primary crystallites (red color) and agglomerates (blue color) is given. For precipitate Z02 both scattering and absorption is governed mainly by agglomerates.
